# Supplementary material for: Approaching Human-Level Forecasting with Language Models
Source: arXiv:2402.18563 source file (2024-02-28)
Supplement: Supplementary file 1 [file evaluation.tex]

\section{Further Details on Ablation Evaluations}
\label{sec:ablate}
We now present $2$ ablated versions of our system. In the first one, we use the optimal hyperparameter configurations and perform retrieval, yet without using a fine-tuned reasoning model. In the second, no retrieval is done, and we simply use GPT-4-1106-Preview to generate forecasts.

% We report the metrics  for each platform and category. This involves the following steps:
% \begin{itemize}
%    \item Brier score calculation:  we calculate the Brier score for each set of predictions within a retrieval index. 
%    \item Averaging Brier scores: We then average these Brier scores across all retrieval indices for each question. This average gives the final Brier score for that particular question.
%    \item Platform and category: Finally, to determine the overall performance per platform and category, we average the final Brier scores of all questions. This same process is replicated for calculating accuracy.
% \end{itemize}

 % We omit the Social Science category, as  no question of the class appears  in the test set.
 
\label{sec:further-eval}
\subsection{Non-fine-tuned System}
\label{sec:non-fine-tune}
\paragraph{Experiment.}
We evaluate our system with a non-fine-tuned reasoning model (GPT-4-1106-Preview), while fixing all other configurations to be the optimal setting that we find (\autoref{sec:optimization}). 
We generate $3$ forecasts for each question, using the top $3$  reasoning prompts we identify (including \autoref{fig:optimal-reasoning-prompt}). We aggregate them taking the trimmed  mean.

\paragraph{Results.}
We compare our system's performance  with human crowd aggregates. 
We find that the non-fine-tuned system is less competitive than our optimal system. See results in \autoref{tab:one-ablation-table}.
% See \autoref{tab:non_finetuned_double} for the full results.

\subsection{Non-retrieval-augmented System}
\label{sec:non-retrieval}
\paragraph{Experiment.}
The evaluation of the non-retrieval-augmented system uses the same method outlined above.  In particular, we use the same reasoning model (GPT-4-1106-Preview), the same   reasoning prompts,  and aggregation method (trimmed mean). The  only difference is that the system    performs no retrieval. 

\paragraph{Results.} 
We observe significant decline in our system's performance.
This suggests the importance of IR in the context of forecasting. See results in \autoref{tab:one-ablation-table}.
% See \autoref{tab:non_finetuned_wo_info_double} for the full results.

% See \autoref{tab:non_finetuned_wo_info_platform} for the results by platform. See \autoref{tab:non_finetuned_wo_info_category} for the results by category. 

% \input{tables/system_eval_without_retrieved_non_finetuned_by_competition}
% \input{tables/system_eval_without_retrieved_non_finetuned_by_category}

% \paragraph{Key takeaways.}
% Our evaluation of the system in both ablated configurations—without a fine-tuned reasoning model and without retrieval augmentation—yields critical insights into the system's performance:
% \begin{enumerate}
%     \item The non-retrieval system performs (scores $0.204$, see \autoref{tab:non_finetuned_wo_info_double}) slightly better than the scratchpad (scores $0.209$, see \autoref{tab:model_comparison}) by $0.005$, due to the utilization of the top-performing prompts from an evaluation of 15 base prompts, in contrast to the basic prompt used for the scratchpad. 
%     \item The retrieval system (scores $0.183$, see \autoref{tab:non_finetuned_double}) significantly outperforms the non-retrieval system (scores $0.204$, see \autoref{tab:non_finetuned_wo_info_double}) by $0.021$ in Brier score. This substantiates the importance of IR in enhancing the forecasting capabilities of our system.
% \end{enumerate}
