# Supplementary material for: Approaching Human-Level Forecasting with Language Models
Source: arXiv:2402.18563 source file (2024-02-28)
Supplement: Supplementary file 4 [file models.tex]

\section{Details about Models and Knowledge Accuracy}
\subsection{Models}
\label{sec:appendix-models}
We give a list of detailed information of the models we use below. The weights of the open models are available publicly on Hugging Face, and we primarily use Together AI's serving API to access them. All cut-offs are based on official statements.

\input{tables/model_source}
% \newpage

\subsection{Knowledge Evaluation by Category}
\label{sec:knowledge-eval}
In our baseline zero-shot prompt evaluations on the test set, we find model exhibit variations in their performance across categories (\autoref{tab:knowledge-accuracy-cate}).

\input{tables/base_eval_zero_shot_by_category}

\input{figures/base_eval_knowledge_prompt}
To explain this,  we  seek to understand models' pre-trained knowledge across categories. In particular, we examine questions from the training and validation sets, all of which have been resolved. We prompt each LM to determine if it can correctly answer the resolved forecasting questions. See \autoref{fig:model-knowledge-eval-prompt} for the knowledge prompt.

\input{tables/base_eval_knowledge_by_category}

\paragraph{The potential for domain-adaptive training.} 
We analyze the correlation between the models' knowledge accuracy   and their Brier scores of the zero-shot prompt evaluation. Notably, in the Politics \& Governance category, there exists a strong negative correlation, while the Education \& Research, Sports, and Other categories display a moderate negative correlation. See the below \autoref{tab:knowledge-zero-shot-correlation} for the correlation table. This negative correlation is expected because a higher knowledge accuracy  should intuitively correspond to a lower Brier score. As a direction for future research, we propose that domain-adaptive training could be employed to enhance forecasting performance in specific categories.

\input{tables/correlation_between_knowledge_and_zero_shot}
